# Supplementary material for: SoK: Anti-Facial Recognition Technology
Source: arXiv:2112.04558 source file (2023-02-15)
Supplement: Supplementary file 1 [file rev_appendix.tex]

\section*{Major Revision Appendix}

A prior version of the paper was submitted to the December 2, 2021 deadline for Oakland 2022. We thank the reviewers for the opportunity to submit a major revision for this paper.  Here, we describe the updates made as part of the major revision resubmission. \erev{Changes made for the major revision are marked in this color.} The requests made by the reviewers are listed below, alongside the corresponding edits and their location in the paper body. 

\begin{packed_enumerate}
    \item {\bf Make the scope of the facial obfuscation systems more focused.} Our revision includes additional text in \S\ref{subsec:litreview} describing both the prevalence of adversarial machine learning (AML)-based AFR tools and the necessity of our work including a few non-AML tools. AFR proposals for stage $\crc{1}$ and $\crcs{2b}$ are inherently non-AML-based, and we believe it is important to consider tools targeting these stages.
    \item {\bf Motivate and explain the 5-step workflow for FR systems, especially how this model is rooted in FR system.} We have added text throughout the paper to clarify this point, especially to \S\ref{sec:back} and \S\ref{sec:stages} to clarify relationship the between stages and FR systems. Additionally, we have introduced notation to draw more explicit links between FR system operational components and targets of AFR systems. Finally, we have updated Figure~\ref{fig:dataflow} to illustrate the links more clearly.
   \item {\bf Make the scope of the threat model more clear}: We have clarified our threat model in two ways. First, we used the newly-introduced notation to formally define the goals of an AFR system, e.g. that an ideal AFR tool counteracting a FR system {G, F, C} will produce $C(F(G(x))) \neq P$. Second, we added explanatory text in the discussion of threat model assumptions to answer questions reviewers had raised (e.g. scope of "image-based" AFR tools).
   \item {\bf Revision needs to give a comprehensive overview of related, published surveys - in particular highly related ones (e.g. Privacy–Enhancing Face Biometrics: A Comprehensive Survey ). A revision needs to clearly differentiate itself from these efforts and describe an independent value}. We have added a discussion in \S\ref{sec:intro} to address related surveys.  These surveys cover topics that are related but orthogonal to the goals of AFR tools.
   \item {\bf Make the distinction between FR systems and Facial verification systems clear in the paper.} We have added text in \S\ref{sec:back} to clarify this distinction. 
   \item {\bf Discuss the trade-off between usability, utility, and privacy properties.} A new technical challenge (TC 3 in~\S\ref{sec:future}) has been added to address this point. 
   \item {\bf Elaborate on the shortcomings of AML-based approaches.} We have addressed this point in two ways. First, we have added short discussion sections at the end of \S\ref{sec:collection}-\S\ref{sec:evade} to illustrate the benefits and shortfalls of existing AFR proposals at each stage. As many proposals fall under the umbrella of AML, these discussion sections highlight their shortcomings. Second, we refined TC 1 in \S\ref{sec:future} to focus explicitly on AML tools for AFR. 
   \item {\bf Be more comprehensive in the literature overview - also drawing more from the substantial work that was presented in the CV community}. Three revisions address this point. First, we added the requested discussion of related survey work. Second, we have added an extended discussion of the challenges of targeting each AFR stage and current progress made by proposals at each stage in \S\ref{sec:collection}-\S\ref{sec:evade}. We believe this provides a much more in-depth study of the AFR stages and current proposals. Finally, we updated Table~\ref{tab:taxonomy} to include new AFR proposals published since our original submission. 
\end{packed_enumerate}

\section*{Changes proposed to reviewers on 03/22/2022}

Before we completed our major revision, we uploaded a list of our proposed changes to the reviewers in the HotCRP system. Below, we include that list (ordered as above) for comparison against the actual changes made. 

\begin{packed_enumerate}
    \item {\bf Make the scope of the facial obfuscation systems more focused.} There were several comments in the reviews about focusing the survey exclusively on AML-based AFR tools. Our revision will emphasize the prevalence of AML-based AFR tools, but AFR tools for stage 1 in our framework are inherently non-AML based. We believe it is important to consider tools operating at stage 1, since data collection is critical for facial recognition. 
    \item {\bf Motivate and explain the 5-step workflow for FR systems, especially how this model is rooted in FR system.} As mentioned briefly above, we will update the paper to include the notation introduced in the rebuttal and emphasize the connection between the FR system workflow and our 5 stages. 
    \item {\bf Make the scope of the threat model more clear}: We will add the notation discussed in the rebuttal throughout the paper to formalize/clarify the 5-step workflow. This notation should also clarify the threat model, e.g. that an ideal AFR tool counteracting a FR system {G, F, C} will produce $C(F(G(x))) \neq P$.  
    \item {\bf Revision needs to give a comprehensive overview of related, published surveys - in particular highly related ones (e.g. Privacy–Enhancing Face Biometrics: A Comprehensive Survey ). A revision needs to clearly differentiate itself from these efforts and describe an independent value}. We will add a section discussing other surveys, including the one mentioned. Overall, we find that existing surveys focus on tools which enable facial recognition while preserving some degree of individual privacy, as opposed to preventing facial recognition altogether (the goal of papers highlighted in this work). We plan to describe this clear distinction, and thus the contribution of our work in systematizing the AFR space.   
    \item {\bf Make the distinction between FR systems and Facial verification systems clear in the paper.} We will update the discussion of FR vs face verification in Section II to clarify this distinction. 
    \item {\bf Discuss the trade-off between usability, utility, and privacy properties.}  We will add technical challenge (TC) in Section X and refine existing text to thoroughly explore this tradeoff. 
    \item {\bf Elaborate on the shortcomings of AML-based approaches.} This text will be added in two places: first, throughout sections V-IX, to denote effective vs ineffective proposals based on the criteria for each stage. We will also add an additional TC (TC 1) in Section XI to discuss the general limitations of AML-based approaches. 
    \item {\bf Be more comprehensive in the literature overview - also drawing more from the substantial work that was presented in the CV community}. We will update Section~\ref{sec:stages} to include more recent work, as well as the surveys previously mentioned. Additionally, as previously requested by the reviewers, we will add more commentary to sections V-IX to highlight more and less successful AFR approaches.
\end{packed_enumerate}
